# Supplementary material for: Nonparametric inference of higher order interaction patterns in networks
Source: arXiv:2403.15635 source file (2024-04-02)
Supplement: Supplementary file 1 [file SI.pdf]

# Supplementary Information for 'Nonparametric inference of higher order interaction patterns in networks'

## 1 Likelihood functions for degree corrected microcanonical subgraph configuration models

Here we briefly review the our derivation of the likelihood for the degree corrected subgraph configuration models given in (1) which are closely related to the model by Karrer and Newman (2). Karrer and Newman describe their model in terms of a generating process that generalizes the stub matching process for the edge configuration model to include higher order atomic subgraphs. Given a set of atoms $M$ and a corresponding atomic degree sequence $\mathbf{d}_{m,i}$ one attaches to every vertex atomic stubs reflecting its atomic degrees. These atomic stubs can be thought of as partial subgraphs such as half edges in the case of edges and corners in the case of triangles. A configuration is then generated by matching these subgraph stubs corresponding to the same atom $m$ in appropriate combinations uniformly at random and connecting them to form $m$-subgraphs until no stubs are left. Given an atomic degree sequence $\mathbf{d}_{m,i}$ the number of distinct matchings is:

$$\Omega_{stub}(\mathbf{d}_{m,i}) = \prod_m \frac{1}{n_m!} \prod_i \frac{(|O_{m,i}|n_m)!}{(|O_{m,i}|!)^{n_m} \prod_v d_{m,i}(v)!}, \tag{1}$$

where $|O_{m,i}|n_m!$ is the number of arrangements of stubs of type $m,i$ and the factor $|O_{m,i}|!^{n_m}$ accounts for the order of the stubs in a matching and $\prod_v d_{m,i}(v)!$ accounts for the fact that stubs attached to the same vertex are equivalent. Finally, $n_m!$ accounts for the possible rearrangements of the subgraphs. Given a set of stubs in certain cases it is possible to create more than one $m$-subgraph that satisfies the constraints on orbits. For instance, there is only one possible way a triangle can be formed on 3 vertices whereas there are 3 different ways a 4-cycle can be formed on 4 vertices. Note that both of these only have one orbit. In this case the subgraph to be formed is chosen uniformly at random. Given the orbit memberships of the vertices there $\mu_m = \prod_i |O_{i,m}|!/|\mathrm{Aut(m)}|$ such distinct $m$-subgraphs that can be formed.

$$\Omega_{subgraph}(\mathbf{d}_{m,i}) = \prod_m \frac{1}{|\mathrm{Aut(m)}|^{n_m} n_m!} \prod_i \frac{(|O_{m,i}|n_m)!}{\prod_v d_{m,i}(v)!}. \tag{2}$$

While the process samples all possible matchings uniformly it also allows for stubs attached to the same vertex to be matched together resulting in a subgraph that is a vertex contraction of $m$. For instance, the vertex contraction of an edge creates a self loop and the vertex contraction of a triangle creates two parallel edge with a self loop on one of its vertices. Moreover, the matching process also allows multiple (parallel) copies of the same subgraph to be created. In other words not all matchings correspond to a valid subgraph configuration in our definition. If one excludes these cases by restarting the generating process whenever they occur every subgraph configuration with atomic degree sequence $\mathbf{d}_{m,i}$ is formed with equal probability. In order to discount for such cases we consider the probability that no stubs of the same vertex are matched together and the probability that no parallel copies of the same subgraph are created during the generation process. The probability that none of the stubs attached to a given vertex $v$ having atomic degree $d_{m,i}(v)$ are matched together is given by:

$$P_c(d_{m,i}(v)) = \prod_m \frac{n_m!}{(n_m - \sum_i d_{m,i}(v))!} \times \prod_i \frac{(|O_{m,i}|n_m - d_{m,i}(v))!|O_{m,i}|^{d_{m,i}(v)}}{(|O_{m,i}|n_m)!}. \tag{3}$$

Expanding the above expression using Stirling's approximation and summing the resulting expression over all vertices we obtain the following overall correction factor:

$$\log(P_c(\mathbf{d}_{m,i})) = -\frac{1}{2}\sum_m \Big[|m|(\frac{\langle(\sum_i d_{m,i})^2\rangle}{\langle\sum_i d_{m,i}\rangle} - 1) - \sum_i\Big(\frac{\langle d_{m,i}^2\rangle}{\langle d_{m,i}\rangle} - 1\Big)\Big], \tag{4}$$

where $\langle d_{m,i}\rangle = \sum_v d_{m,i}(v)/N$. Although the assumption of independence is not rigorous the dependence in general is weak and the independence assumption is known to produce results that are consistent with more rigorous analyses for sparse simple graphs that is when $M$ consists of only the single edge (3).

In order to account for the cases where more than one copy of a subgraph is generated we consider the probability $P_2(s)$ that at least 2 copies of a certain $m$-subgraph $s$ being created during the matching process. For an $m$-subgraph with orbits $O_{m,i}(s)$ we have:

$$\begin{aligned} P_2(s) = &\frac{|\mathrm{Aut(m)}|^2}{2}\frac{n_m!}{(n_m-2)!}\prod_j \frac{(|O_{m,j}|(n_m-2))!}{(|O_{m,j}|n_m)!} \\ &\times \prod_{i,v|v\in O_{m,i}(s)} \frac{d_{m,i}(v)!}{(d_{m,i}(v)-2)!}. \end{aligned} \tag{5}$$

Where we assume that $d_{m,i}(v) \geq 2$ for all vertices of $s$, since $P_2(s) = 0$ otherwise. The probability of there being no multiple copies of $s$ is simply $1 - P_2(s)$. Assuming independence between all such subgraphs one obtains the following correction factor:

$$\begin{aligned} \log(P_{ml}(\mathbf{d}_{m,i})) &= \sum_{s\in\mathcal{H}_N(m)} \log(1-P_2(s)) \\ &\simeq -\frac{|\mathrm{Aut(m)}|n_m^2}{2}\prod_i \frac{1}{(n_m|O_{m,i}|)^{|O_{m,i}|}}\Big(\frac{\langle d_{m,i}^2\rangle}{\langle d_{m,i}\rangle} - 1\Big)^{|O_{m,i}|}. \end{aligned} \tag{6}$$

Where we assumed $P_2(s) \ll 1$ so that $\log(1-P_2(s)) \simeq -P_2(s)$.

Finally, we obtain the overall expression for the log likelihood by considering $-\log(P(\mathbf{d}_{m,i})) = \log\big(\Omega(\mathbf{d}_{m,i})P_c(\mathbf{d}_{m,i})P_{ml}(\mathbf{d}_{m,i})\big)$:

$$\begin{aligned} -\log(P(\mathbf{d}_{m,i})) = \sum_m \Bigg[ &-\log(n_m!) - n_m\log(|\mathrm{Aut(m)}|) + \sum_i\Big[\log((|O_{m,i}|n_m)!) - \sum_v \log(d_{m,i}(v)!)\Big] \\ -\frac{|\mathrm{Aut(m)}|n_m^2}{2}\prod_i \frac{1}{(n_m|O_{m,i}|)^{|O_{m,i}|}}\Big(\frac{\langle d_{m,i}^2\rangle}{\langle d_{m,i}\rangle} - 1\Big)^{|O_{m,i}|} &- \frac{1}{2}\Big[|m|(\frac{\langle(\sum_i d_{m,i})^2\rangle}{\langle\sum_i d_{m,i}\rangle} - 1) - \sum_i\Big(\frac{\langle d_{m,i}^2\rangle}{\langle d_{m,i}\rangle} - 1\Big)\Big]\Bigg]. \end{aligned} \tag{7}$$

This expression reduces to known expressions for entropy of microcanonical ensembles of graphs with a given degree distribution (3; 4) for directed and undirected graphs when $M$ contains only the single edge atom.

## 1.1 The likelihood for coarse grained models

The likelihood of the coarse grained models can be obtained following the same procedure as in the orbit degree model. The coarse grained model we use can be seen as the result of aggregating the degree sequences of groups of orbits. In the simplest case where we aggregate two orbits $m_1, i$ and $m_2, j$ we have :

$$d(v) = d_{m_1,i}(v) + d_{m_2,j}(v). \tag{8}$$

where $m_2$ might be the same as $m_1$. Such ensembles can be obtained by treating the stubs of the combined orbits as a single type during the generation process. In this case one has to replace the two factors corresponding to these orbits in Eq. (2) by:

$$\frac{(|O_{m_1,i}|n_{m_1} + |O_{m_2,j}|n_{m_2})!}{\prod_v d(v)!}. \tag{9}$$

The equivalent of $P_c$ (Eq.4) can be obtained by assuming that the orbit degree $d_{m_1,i}$ follows a binomial distribution in the interval $[0, k(v)]$ with probability $p_{m_1,i} = \frac{|O_{m_1,i}|n_{m_1}}{|O_{m_1,i}|n_{m_1}+|O_{m_2,j}|n_{m_2}}$. Which yields $\langle d_{m,i}\rangle = p_{m,i}\langle d\rangle$ and $\langle d^2_{m,i}\rangle = p^2_{m,i}\langle d(d-1)\rangle + p_{m,i}\langle d\rangle$. Similarly the correction factor for multiple subgraphs (Eq. (6)) can be obtained by replacing the factor corresponding to $O_{m_1,i}$ by:

$$\frac{1}{(|O_{m_1,i}|n_{m_1} + |O_{m_2,j}|n_{m_2})^{|O_{m_1,i}|}}\left(\frac{\langle d^2\rangle}{\langle d\rangle} - 1\right)^{|O_{m_1,i}|}. \tag{10}$$

The final expression for the entropy can be obtained by making the same substitutions for $(m_2, j)$ as well. In this case the analogue of Eq.2 can be obtained by considering a total number of $\sum_m |m|n_m$ stubs which are matched into subsets according to $\mathbf{n_m}$:

$$\Omega_{TD}(\mathbf{d}, M, \mathbf{n_m}) = \frac{(\sum_m |m|n_m)!}{\prod_m (|m|!)^{n_m} n_m! \prod_v d(v)!}\prod_m \left(\frac{|m|!}{|Aut(m)|}\right)^{n_m}. \tag{11}$$

Orbit aggregation is commutative and generalizes to the case where multiple disjoint subsets of orbits are aggregated at once.

#### 1.1.1 Atomic degree model

First we consider the microcanonical ensemble where all the orbits corresponding to the same $m$ are aggregated:

$$d_m(v) = \sum_i d_{m,i}(v), \tag{12}$$

for all $m \in M$. Note that this is equivalent to removing the distinction between orbits of the same atom. Applying the corresponding transformations derived above we obtain the following expression for the entropy:

$$\begin{aligned} S(M, \mathbf{d}_m) = \sum_m \Bigg[ &-\log(n_m!) - n_m \log(|\mathrm{Aut(m)}|) + \log((|m|n_m)!) - \\ \sum_v \log(d_m(v)!) &- \frac{|\mathrm{Aut(m)}|n_m^2}{2(n_m|m|)^{|m|}}\left(\frac{\langle d_m^2\rangle}{\langle d_m\rangle} - 1\right)^{|m|} - \frac{|m|-1}{2}\left(\frac{\langle d_m^2\rangle}{\langle d_m\rangle} - 1\right)\Bigg], \end{aligned} \tag{13}$$

where we used the fact that $\sum_i |O_{m,i}| = |m|$. Note that this is the same expression one would obtain if all atoms had a single orbit.

#### 1.1.2 Total degree model

In the total degree model only the total number of atoms attached to each vertex is conserved which corresponds to aggregating atomic degrees of all orbits into a single degree distribution:

$$d(v) = \sum_{m\in M}\sum_i d_{m,i}(v). \tag{14}$$

Using the transformations derived previously the entropy can be found to be:

$$\begin{aligned} S(M, \mathbf{n}_m, \mathbf{d}) = \log((\sum_m |m|n_m)!) - \sum_v \log(d(v)!) - \sum_m \Bigg[ &\log(n_m!) + n_m \log(|\mathrm{Aut(m)}|) \\ + \frac{|\mathrm{Aut(m)}|n_m^2}{2(\sum_{m'}|m'|n_{m'})^{|m|}}\left(\frac{\langle d^2\rangle}{\langle d\rangle} - 1\right)^{|m|} &+ \frac{|m|-1}{2}\frac{|m|n_m}{(\sum_{m'}|m'|n_{m'})}\left(\frac{\langle d^2\rangle}{\langle d\rangle} - 1\right)\Bigg]. \end{aligned} \tag{15}$$

This model has only a single degree sequence as its parameter and hence the expression above and Eq. (7), Eq. (13) all become equivalent when the model has a single atom with one orbit.

### 1.1.3 Directed degree model

In the case of the directed degree model we group orbits according to their in and out degrees in to three different groups i.e orbits with only incoming edges $d_{in}(v) = \sum_{m,i|d_{out}(O_{m,i})=0} d_{m,i}(v)$, only out going edges $d_{out}(v) = \sum_{m,i|d_{in}(O_{m,i})=0} d_{m,i}(v)$ and those which have both in and out going edges $d_{io}(v) = \sum_{m,i|d_{out}(O_{m,i})\neq 0, d_{in}(O_{m,i})\neq 0} d_{m,i}(v)$. For each $m$ we group its orbits in the same way and these groups as $O_{m,in}$, $O_{m,out}$ and $O_{m,io}$, respectively. For each of these groups we denote the total we consider the number of vertices in each type of orbit which we denote as $|O_{m,in}| = \sum_{O\in O_{m,in}} |O|$, $|O_{m,out}| = \sum_{O\in O_{m,out}} |O|$ and $|O_{m,io}| = \sum_{O\in O_{m,io}} |O|$, respectively. Following the same procedure as for the other coarse grained ensembles we obtain the following expression for the entropy:

$$
\begin{aligned}
S(M,\mathbf{n}_m,\mathbf{d}) = & \sum_{t\in\{in,out,io\}} \Big[\log(D_t!) - \sum_v \log(d_t(v)!)\Big] - \sum_m \Big[\log(n_m!) + n_m \log(|\mathrm{Aut(m)}|) \\
& + \frac{|\mathrm{Aut(m)}| n_m^2}{2} \prod_{t\in\{in,out,io\}} \frac{1}{(\sum_{m'} |O_{m',t}| n_{m'})^{|O_{m,t}|}} \Big(\frac{\langle d_t^2\rangle}{\langle d_t\rangle} - 1\Big)^{|O_{m,t}|} \\
& + \frac{1}{2}\Big[|m| \frac{|m| n_m}{\sum_{m'} |m'| n_{m'}} \Big(\frac{\langle(\sum_t d_t)^2\rangle}{\langle \sum_t d_t\rangle} - 1\Big) - \sum_t \frac{|O_{m,t}| n_m}{(\sum_{m'} |O_{m',t}| n_{m'})} \Big(\frac{\langle d_t^2\rangle}{\langle d_t\rangle} - 1\Big)\Big]\Big].
\end{aligned}
\tag{16}
$$

# 2 Details of priors

## 2.1 Priors on atoms

The identification of a suitable set of atoms is one of the the most challenging aspect of inferring subgraph configurations. In order to allow for the detection of atoms ideally the set of potential motifs should be kept as general as possible. In practice though one is faced with several problems related to the fact hat the number of motifs increases super-exponentially with size of the motifs and the computational complexity of finding subgraphs. Therefore, in most practical settings one is forced to restrict the size of atoms included in the analysis resulting in finite sets of candidate motifs. We initially consider the case where the set of possible motifs is finite but later also discuss the case where the set of candidate motifs is infinite.

### 2.1.1 Finite sets of motifs

We first consider the the setting where the possible patterns in $M$ are restricted to a finite set $\mathcal{M}$, which call the set of candidate patterns.

**Uniform prior** The simplest prior one can consider in the case of a finite set of candidate patterns is to assume that all non-empty subsets of $\mathcal{M}$ are equally likely resulting in a prior $P(M) = (2^{|\mathcal{M}|} - 1)^{-1}$.

**Hyper-prior** Under the uniform prior the expected number of patterns in $M$ is $|\mathcal{M}|/2$ which is quite unrealistic for large sets of candidate motifs that can easily exceed the size of the network. Alternatively, one could assume a uniform prior that is conditioned on the number of patterns in $M$, together with a uniform prior on such sets. Resulting in a prior of the form:

$$
P(M) = P(|M|)\binom{|\mathcal{M}|}{|M|}^{-1},
$$

where $P(|M|)$ is a prior on the size of $M$. One typical choice is $P(|M|) \propto 1/|M|$.

On the other hand, both the uniform prior and the hyper-prior assign equal probability to all patterns in a given candidate set. However, intuitively it could be argued that simple patterns should be considered more likely to appear in a network than complex ones. For instance it would be highly surprising if a certain network could be modelled by a set of patterns that does not include the single edge motif.

**Independent prior** Given an finite set of candidates we assume that motifs occur independently with probabilities $p_m \in (0,1)$. Where $p_m$ is chosen such as to reflect the complexity of $m$. Resulting in a prior of the form:

$$P(M) = \prod_{m \in M} p_m \times \prod_{m \notin M} (1 - p_m). \tag{17}$$

We discuss the problem of assigning probabilities to atoms in the context of infinite sets of candidate motifs.

### 2.1.2 Infinite sets

Ideally one would like to have a prior that allows arbitrary patterns to be learned from the data. In this context assuming that patterns are drawn from an infinite set of potential patterns proves to be a useful guide in formulating priors that favours simpler patterns over more complex ones. Moreover, in the infinite case the assumption that all patterns are equiprobable results in ill defined priors.

**Infinite sets of candidate motifs and universal priors** In the case of infinite motif sets we assume a prior of the form given by Eq.17. In the case of infinite candidate sets we require that $\sum_{m \in \mathcal{M}} p_m = \alpha < \infty$ in order to ensure that the prior is proper. This conditions also insures that the expected number of motifs in $M$ is finite. We write the prior in the following, more convenient, form:

$$P(M) = Z \times \prod_{m \in M} \frac{p_m}{1 - p_m}, \tag{18}$$

where $Z = \prod_{m \in \mathcal{M}} (1 - p_m)$ and $Z$ is finite and non-zero as a result of $\sum_{m \in \mathcal{M}} p_m = \alpha < \infty$.

Without loss of generality we assume that the elements of $\mathcal{M}$ are ordered according to $p_m$ (i.e. $p_{m+1} \leq p_m$). In the case of infinite sets the uniform prior is not well defined and hence we follow the approach of Rissanen (5) and require that our prior has infinite entropy i.e we require:

$$\sum p_m = \alpha < \infty, \tag{19}$$

$$H(P_M) = \sum h(p_m) = \infty, \tag{20}$$

where $h(p_m) = -p_m log(p_m) - (1 - p_m) log(1 - p_m)$ is the binary entropy. The last condition is analogous to the prior being non-informative. Making use of the expansion $h(p) = -p \log(\frac{p}{e}) + O(p^2)$ the last condition becomes equivalent to $H(p_m) = \sum_m -p_m \log(p_m) = \infty$. Putting aside the normalization condition of Eq.19 this reduces to the definition of Rissanen (5) of a universal prior for integers. The above equations have no unique solution but such priors can be shown to agree with respect to their leading order term. Consequently, one way of constructing a prior that satisfies the above conditions is to order motifs (i.e. map them on to integers) in a way that reflects our prior knowledge regarding the likelihoods of motifs and set $p_m$ to be equal to the probability of the integer index $n(m)$ of $m$ under a universal prior for the integers for instance $p_m = 2^{-\log^*(n(m))+c}$.

Having defined a prior with the desired properties one is left with the task of ordering motifs. We first define one such possible ordering for the most general case where one considers the space of all (connected) motifs. Such an order automatically induces an ordering on more restricted subsets of motifs such as cliques, stars, cycles etc. For this we consider an ordering in which motifs are initially ordered according to the number of nodes and then the number of edges. Motifs having the same number of nodes and edges can then ordered on the basis of their adjacency matrices. For instance given a motif $m$ one can consider the all adjacency matrices representing labelled graphs in the isomorphism class $m$ and order these lexicographically by concatenating the rows of the adjacency matrix. Finally, one than chooses the adjacency matrix with lowest lexicographical rank as the representation of $m$. Motifs having the same number of nodes and edges are then ranked lexicographically according to these representations. Note that this ordering is well defined and is independent of the initial adjacency matrix chosen to represent $m$. Here, we should however note that mapping an arbitrary labelled graph to its integer index under this (or any other) ordering is bound to be computationally challenging because it implicitly requires solving the graph isomorphism problem. On the other hand, if the set of motifs consists of special classes motifs such as cliques, bi-cliques, cycles, stars etc. ordering these becomes straightforward.

Another more practical ordering can be obtained by considering a computer program that sequentially generates all motifs in the class under consideration (such as the *nauty* package) sequentially and equate the ordering of motifs to the order they are generated by the given computer program. In our implementation we generate candidate motifs using the *nauty* tool-box where motifs are generated/ordered according to the number vertices, number of edges and canonical labelling (6). The code for generating/labelling motifs is included in the software package that accompanies the paper.

The priors for infinite sets of motifs also offer a principled and convenient way of constructing priors for finite sets of candidate motifs. The only difference being in the normalization constant $Z$ in Eq.18.

**Choosing candidate motifs** When the goal of the inference is to identify characteristics connectivity patterns the set of candidate motifs should ideally be kept as general as possible. However, in practice the fact that the number of potential motifs grows super exponentially with size and the problem of finding such subgraphs in the network pose computational challenges. Consequently, in practice the set of candidate motifs is dictated by computational resources. In general algorithms that involve finding subgraphs for a given set of candidates can only be feasibly applied to motifs with up to 8 nodes in the case undirected networks and to motifs with up to 5 nodes in the case of directed networks assuming $G$ is relatively sparse and has less than $10^4$ nodes.

On the other hand, prior knowledge on the structure of the network might lead one to consider motif sub-classes that are known to be relevant to the structure of the network for instance cliques in the case of collaboration networks or directed bipartite cliques in the case of chemical reaction networks. In such cases all instances it might be possible to enumerate all candidate subgraphs efficiently regardless of size.

# 3 Implementation details

In the following we present a detailed description of the inference algorithm.

Due to the NP-completeness of finding a MAP configuration we rely on a greedy heuristic that is inspired by the greedy heuristic for set covering problems (7). Starting from an empty configuration $C_0$, at each step the algorithm identifies the atom whose copies are most effective in covering edges not yet in the configuration where the effectiveness of a set of $m$ subgraphs $C_m$ is measured in terms of the description length per edge. The effectiveness of atom $m$ in covering edges at iteration $t$ of the algorithm is determined by finding a set of $m$-subgraphs $C_m$ that minimizes:

$$\sigma_{m,t} = \frac{\Delta\Sigma_t(C_m)}{|(E(G) - E(C_t)) \cap E(C_m)|}, \tag{21}$$

where $E(C_t)$ is the set of edges covered by the configuration $C_t$ at iteration $t$, $E(C_m)$ is the set of edges contained in the subgraphs in $C_m$ and $\Delta\Sigma_t(C)$ is the change in $\Sigma$ when $C_m$ is added to the current state i.e. $\Sigma(C_t \cup C_m) - \Sigma(C_t)$. Finding such a set of $m$-subgraphs that minimizes $\sigma$ is in itself a non-trivial problem which we approximate using a heuristic that seeks to identify a maximum set of edge independent $m$-subgraphs on the graph $G_t$ with edges $E_t = E(G) - E(C_t)$. For this, the algorithm iteratively finds an $m$-subgraph in $G_t$ adds it to $C_m$ and removes the edges of the found subgraph from $G_t$ until $G_t$ contains no more copies of $m$. To maximize the number of non-intersecting $m$-subgraphs found, we order vertices according to their degree which gives subgraphs on lower degree vertices priority.

Once the algorithm finds an optimal $C_m$ for all $m \in \mathcal{M}$ we check whether $C_t + C_m$ has lower DL than $C_t$. Here the DL of an incomplete configuration $C$ is calculated by completing it through the addition of single edge subgraphs that correspond to the edges of $G$ that are not contained in any of the subgraphs in $C_t$. This is done because the cost function under consideration is nonlinear and in general adding a certain $C_m$ to the configuration $C_t$ lowers the efficiency of other atoms in the next step which in certain cases can lead to sub-optimal solutions. In addition, we also require that $C_m$ contains at least 2 copies of $m$. After these checks the algorithm selects the $C_m$ that minimizes $\sigma_{m,t}$ which is then added to $C_t$ to obtain $C_{t+1} = C_t \cup C_m$. This procedure is then repeated until all edges of $G$ are covered (i.e. when $\bigcup_{s\in C_n} E(s) = E(G)$) which in general occurs when the most effective atom is the single edge.

# 4 Synthetic data sets

## 4.1 Generation of subgraph configuration

Although the stub matching process described in the main text can be used to generate random subgraph configurations with a given set of atom and degree sequence, in practice the procedure might be rather inefficient due to the creation of parallel subgraphs and the stubs of the same vertex being matched together. However, if one is given a subgraph configuration $C$ that already satisfies a set of desired constraints a randomized configuration can be obtained by randomly rewiring/shuffling the subgraphs in $C$ in a way that preserves the desired constraints on atomic degrees, similar to what one would do in randomizing a graph while keeping its degree sequence fixed.

In the case of subgraph configurations the swapping procedure is defined in terms of orbits of subgraphs. In general given two subgraphs $s_1$ and $s_2$ which are defined in terms of embeddings of the respective (labelled) motif $m$ i.e. $s_{1,i} = \{v_{1,i}\}$ and $s_{2,i} = \{v_{2,i}\}$, respectively, where $v_{1,i}$ is the image of the $i^{th}$ vertex of $m$ in its embedding. A corner swap corresponding to orbit $O_{m,o}$ swaps $s_{1,k}$ and $s_{2,l}$ where both $k$ and $l$ are in $\in O_{m,o}$ resulting in two new $m$-subgraphs $s'_1$ and $s'_2$ with embeddings $s'_{1,i} = s_{1,i}$ for $i \neq k$ and $s'_{1,k} = s_{2,l}$ and $s'_{1,i} = s_{1,i}$ for $i \neq l$ and $s'_{2,l} = s_{1,k}$. It is straightforward to show that this swapping operation conserves the orbit degree sequence of the configuration provided that the operation does not create any vertex contracted or parallel subgraphs.

The defined swapping procedure includes operations that leave the configuration unchanged. For instance a swapping operation can match a certain subgraph on to itself if $s_1 = s_2$. Similarly, if $s_{1,k}$ and $s_{2,l}$ happen to be the same vertex of $G$ the swapping operation would leave the both of the subgraphs unchanged. In general we will assume that such moves are not allowed. Similarly we do not allow moves that would more that one corner of a subgraph to the same vertex which would result in a vertex contraction of the subgraph. Note that however the allowed moves do not exclude the possibility that $s_1 = s_2$ which allows for different configurations of $m$ to be formed on a given set of vertices for instance the various configurations a 4-cycle can have on 4 vertices.

The swapping operation can be generalized to other model variants by allowing the mixing of orbits that correspond to the same component of the atomic degree sequence under consideration. For instance, in the total degree model where the orbits of all atoms are aggregated together any pair of corners can be swapped regardless of the type of subgraph they are part of.

Finally, the randomization proceeds by picking pairs of compatible corners uniformly at random and then swapping them - if such a move is allowed. Repeating this procedure for all components sufficiently many times is then expected to yield a random configuration that satisfies the desired constraints.

### 4.1.1 Generation of atomic degree sequences

We generate atomic degree sequences using the following procedure. We generate propensities of nodes to attract each orbit $O_{m,i}$ for a given component by sampling a distribution $\mu$ independently $N$ times resulting in a sequence of degree strengths $\mu_{m,i}(v)$ for each orbit. Given the counts of atoms $n_m$ we obtain a degree sequence $d_{m,i}$ by sampling the distribution over $[1, N]$ where the probability of choosing a vertex $v$ is given by $p_v = \mu(v)/\sum_{j=1}^{N} \mu(v)$, $|O_{m,i}|n_m$ times, independently. Degrees sequences corresponding to other model variants can also generated following the same procedure.

The synthetic data sets we consider were generated by first generating a subgraph configuration via stub matching while allowing parallel and vertex contracted subgraphs. This configuration is the shuffled via corner swapping which will in general removes parallel and vertex contracted subgraphs. The number of swapping steps was chosen to be 50 times the total degree of each component. For instance in the case of the orbit degree model each component $d_{m,i}$ has total degree $|O_{m,i}|n_m$. The code for generating and shuffling subgraph configurations is provided as part of our implementation.

## 4.2 Empirical results for synthetic networks with higher order interactions

Results for synthetic networks are given in Table 1. The accuracy of the method in identifying the underlying subgraph configurations varies slightly depending on the difficulty of the infer-

ence problem and in two of the examples the method identifies extra atoms not present in the generative model though the extra subgraphs correspond to a very small fraction of the graph. In general the discrepancy between theoretical and inferred subgraph configurations can be attributed to the algorithm not finding the optimal configuration as can be confirmed by comparing the description lengths of the inferred and ground truth configurations.

Synthetic benchmarks also illustrate the importance of model selection in inferring subgraph configurations. For instance we find that using homogeneous models to fit degree corrected models with a highly skewed degree distribution can result in the identification of spurious atoms. Similar results hold for networks with heterogeneous degree distributions that were generated using model that only contain edges (See Sec.4.3). Note that in all considered cases the model selection identifies the correct model class and recovers the underlying subgraph configuration to a high degree of accuracy.

| N=2.000 E=4.500 Orbit Degree Model | | | | | | | | | |
|---|---|---|---|---|---|---|---|---|---|
| Atoms | 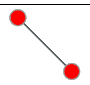 | 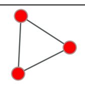 | | | | | | | |
| $n_m$ (Model) | 1500 | 1000 | | | | | | | |
| $n_m$ (Infered) | 1506 | 998 | | | | | | | |
| N=2,000 E=5,100 Total Degree Model | | | | | | | | | |
| Atom | 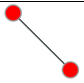 | 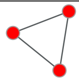 | 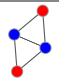 | 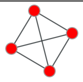 | 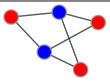 | 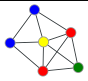 | 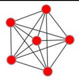 | 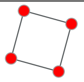 | 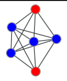 |
| $n_m$ (Model) | 500 | 100 | 100 | 100 | 100 | 100 | 100 | | |
| $n_m$ (Infered) | 561 | 101 | 102 | 92 | 93 | 95 | 97 | 8 | 3 |
| N=2.000 E=3.000 Orbit Degree Model | | | | | | | | | |
| Atom | 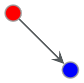 | 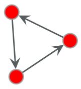 | 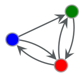 | 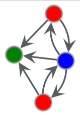 | 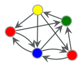 | 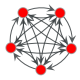 | | | |
| $n_m$ (Model) | 500 | 100 | 100 | 100 | 100 | 25 | | | |
| $n_m$ (Infered) | 500 | 100 | 100 | 100 | 100 | 25 | | | |
| N=1.000 E=3.600 Total Degree Model | | | | | | | | | |
| Atom | 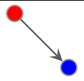 | 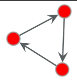 | 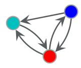 | 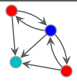 | 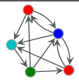 | 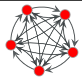 | 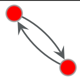 | | |
| $n_m$ (Model) | 500 | 100 | 100 | 100 | 100 | 25 | 0 | | |
| $n_m$ (Infered) | 512 | 100 | 98 | 98 | 100 | 25 | 6 | | |

Table 1: Atoms and their respective counts found the inferred subgraph configurations. Counts corresponding to generated subgraph configurations and the inferred are given in the $n_m(Model)$ and $n_m(Inferred)$ rows respectively.For the degree distributions of synthetic networks a Zipf distribution with exponent 3 was used.

## 4.3 Synthetic networks without higher order interactions

We also tested the method on synthetic networks generated from the preferential attachment model by Barabasi and Albert(8) and it's directed variant aka the Price model as well as the edge configuration model and Erdös-Rényi (ER)(9) random graphs.

We consider ER graphs with 1000 vertices and average degrees of 2,5 and 10. For ER graphs the configuration consisting of all edges is selected for all model variants and the homogeneous model is favoured by model selection.

Next we considered realizations of the BA and Price models $N = 1000$ vertices with $k = 4$. We also consider configuration models corresponding to the same degree sequence as the preferential attachment networks which we obtained by shuffling edges. In the case of these networks which have power law type degree distributions we find that using the non degree corrected models for inference leads to the identification of spurious atomic subgraphs. Nevertheless when model selection is taken into account the method clearly identifies the configuration consisting only of edges the corresponds to the degree corrected model as the better solution highlighting the im-

| | | | | | | | | | |
|---|---|---|---|---|---|---|---|---|---|
| BA model (k=4), N=1.000, E=3.990 | | | | | | | | | |
| Atom | 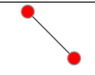 | 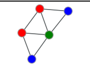 | 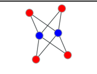 | 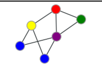 | 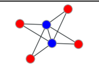 | 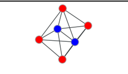 | | | |
| $n_m$ | 3358 | 9 | 29 | 22 | 15 | 2 | | | |
| Configuration Model, N=1.000, E=3.990 | | | | | | | | | |
| Atom | 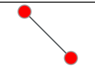 | 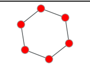 | 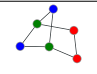 | 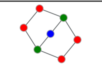 | 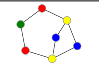 | 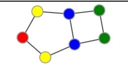 | 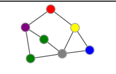 | 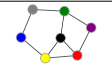 | 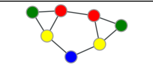 |
| $n_m$ | 2402 | 135 | 34 | 48 | 19 | 18 | 15 | 11 | 4 |
| Price Model (k=4), N=1.000, E=3.990 | | | | | | | | | |
| Atom | 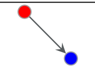 | 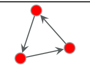 | 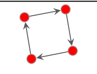 | 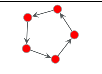 | 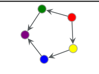 | 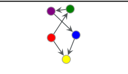 | 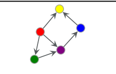 | 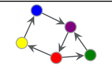 | |
| $n_m$ | 2424 | 9 | 46 | 58 | 85 | 32 | 9 | 6 | |
| Directed CM, N=1.000, E=3.990 | | | | | | | | | |
| Atom | 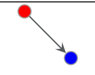 | 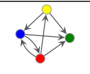 | 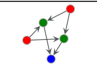 | 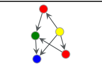 | 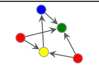 | 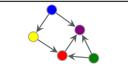 | 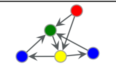 | 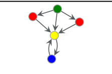 | 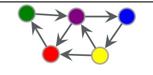 |
| $n_m$ | 3344 | 4 | 24 | 23 | 12 | 16 | 10 | 8 | 6 |

Table 2: Details of subgraph configurations inferred using the non-degree-corrected/homogeneous models for networks generated using the BA model and the Price model for k=4 and their configuration model counterparts. Note that the when based on the degree-corrected models the method identifies correctly identifies the configuration consisting of edges only which also has shorter DL.

portance of using degree corrected models when performing inference on networks with highly heterogeneous degree distributions. The atoms identified by the non degree corrected / homogeneous models in networks generated by the BA and configuration models are given in Table 2.

# 5 Additional results for empirical networks

## 5.1 Network science collaboration network

Fig. 1 shows the network science collaboration network including its disconnected components.

## 5.2 C.elegans neural networks

### 5.2.1 C.elegans Synaptic network (male)

To complement the results presented for th network of synaptic connections in the adult hermaphrodite worms C. elegans we here present the analogous analysis of the network on the male adult of C.elegans. This network has 575 nodes and 5,246 directed edges. The MAP configuration of the network 31 nontrivial atoms that cover approximately 75% of edges. Similar to hermaphrodite network we find that the MAP configuration contains a large number of bi-fan motifs (Atom 4 and 5 in Table 3) and multiple motifs that correspond to various combinations of feed–forward–loops (Atoms 1,8,11,12 and 15 in Table 3). As well as atoms resulting from symmetric combinations of the triangular connection pattern ($A \longleftrightarrow B$, $C \rightarrow A$, $C \rightarrow B$) i.e. atoms 10, 13, 21,23 and 28 in Table 3. Finally, we also observe atoms containing chains and cycles of bidirectional edges such as the atoms 3,16,24,25 and 26 in Table 3 and as well as dense motifs of bidirectional edges including directed cliques (Atoms 29,30 and 31 in Table 3).

### 5.2.2 Gap junction networks

For the gap junction networks we obtain quantitatively similar results for both sexes. The atoms in the MAP configurations of both networks (see Table 5.2.2 and 5.2.2) cover about 65% of edges in both networks. The atoms in the MAP configurations consist mainly of triangles and 4 cy-

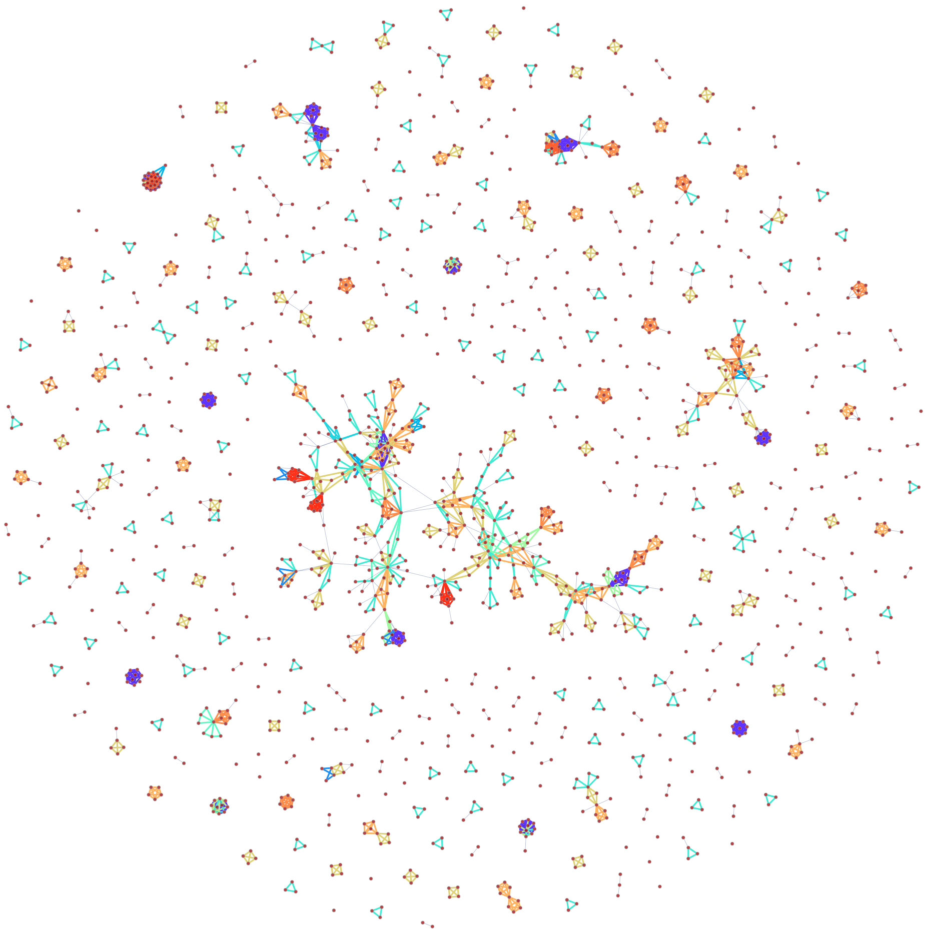

Figure 1: The network science collaboration network including all disconnected component. Edge colors indicate the type of atom edges are covered by in the MAP configuration.

| $m$ | 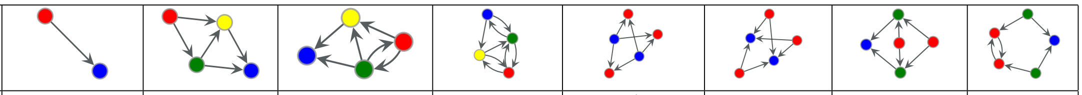 | | | | | | | |
|---|---|---|---|---|---|---|---|---|
| Id | 0 | 1 | 2 | 3 | 4 | 5 | 6 | 7 |
| $n_m$ | 1307 | 16 | 6 | 6 | 118 | 17 | 11 | 12 |
| $m$ | 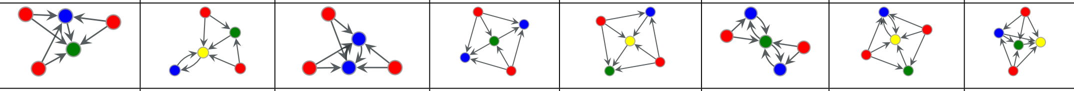 | | | | | | | |
| Id | 8 | 9 | 10 | 11 | 12 | 13 | 14 | 15 |
| $n_m$ | 28 | 8 | 12 | 20 | 14 | 5 | 21 | 15 |
| $m$ | 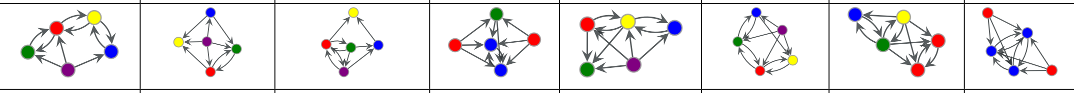 | | | | | | | |
| Id | 16 | 17 | 18 | 19 | 20 | 21 | 22 | 23 |
| $n_m$ | 10 | 4 | 4 | 14 | 16 | 13 | 3 | 17 |
| $m$ | 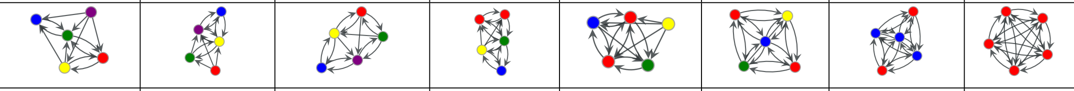 | | | | | | | |
| Id | 24 | 25 | 26 | 27 | 28 | 29 | 30 | 31 |
| $n_m$ | 16 | 6 | 7 | 8 | 9 | 9 | 7 | 6 |

Table 3: Atoms found in the MAP configurations of the network of synaptic connections of the male C.elegans together with their respective counts ($n_m$).

| $m$ | 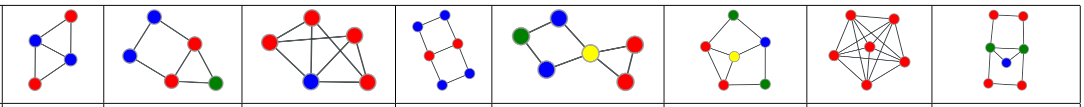 | | | | | | | |
|---|---|---|---|---|---|---|---|---|
| Id | 1 | 2 | 3 | 4 | 5 | 6 | 7 | 8 |
| $n_m$ | 20 | 9 | 2 | 8 | 5 | 8 | 4 | 5 |
| $m$ | 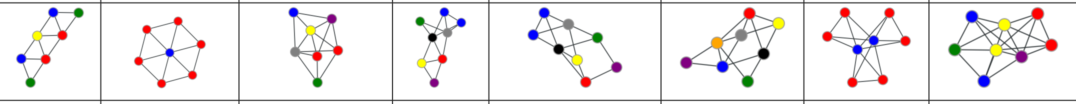 | | | | | | | |
| Id | 9 | 10 | 11 | 12 | 13 | 14 | 15 | 16 |
| $n_m$ | 5 | 4 | 7 | 5 | 2 | 5 | 3 | 3 |

Table 4: Atoms found in the MAP configurations of the gap juction network of the hermaphrodite C.elegans together with their respective counts in the MAP configuration ($n_m$).

cles and regular combinations of these as well as cliques of various sizes. In addition, the MAP configurations also contain several large, sparse and irregular patterns.

### 5.2.3 C.elegans neuronal network(1986)

Thi version of the neural network of C.elegans contains 297 neurons and 2359 edges representing synaptic connections (10). We find that the MAP configuration of the C. elegans network contains 12 non-trivial patterns which cover approximately 40% of the edges. In the C.elegans neural network we recover atoms (Table 5.2.3) that consists of combinations of the feed-forward-loop and variants of the FFL motif where one of the edges is bidirectional. In addition we also observe motifs that contain long chains of bidirectional edges.

## 5.3 Metabolic networks

We finally consider a collection of 43 metabolic networks from (11). We find that the MAP configurations of metabolic networks contain a total of 27 different non-trivial atoms. Moreover, more than 70% of the edges in all networks are covered by non trivial patterns in their respective MAP-configurations.

In order to quantify the relative significance of atoms found in the inferred configurations we use the normalized $c$-score (12). The $c$-score is defined on the basis of the increase in $\Sigma$ when the

| | | | | | | |
|---|---|---|---|---|---|---|
| Atom | 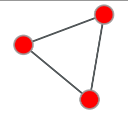 | 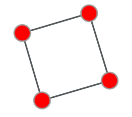 | 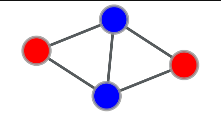 | 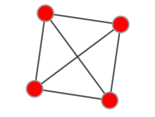 | 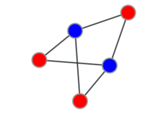 | 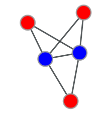 |
| Id | 1 | 2 | 3 | 4 | 5 | 6 |
| $n_m$ | 32 | 26 | 21 | 5 | 3 | 5 |
| Atom | 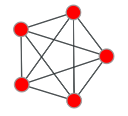 | 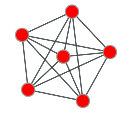 | 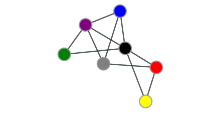 | 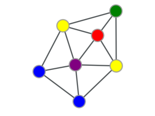 | 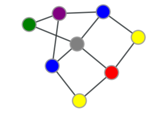 | 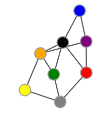 |
| Id | 7 | 8 | 9 | 10 | 11 | 12 |
| $n_m$ | 5 | 4 | 8 | 8 | 8 | 6 |
| Atom | 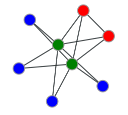 | 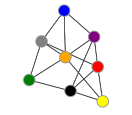 | 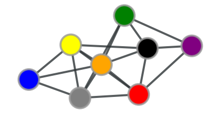 | 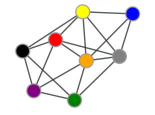 | 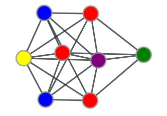 | 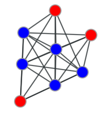 |
| Id | 13 | 14 | 15 | 16 | 17 | 18 |
| $n_m$ | 3 | 2 | 5 | 2 | 3 | 2 |

Table 5: Atoms in the subgraph MAP-configuration of the gap juction network of the male C.elegans and their respective frequencies ($n_m$).

| | | | | | | |
|---|---|---|---|---|---|---|
| Atom | 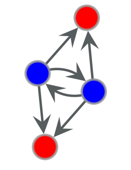 | 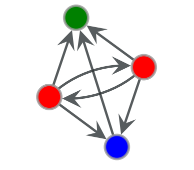 | 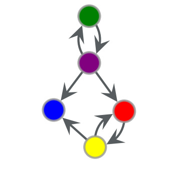 | 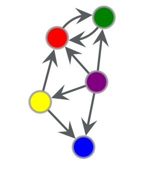 | 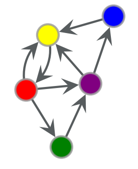 | 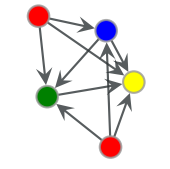 |
| $n_m$ | 8 | 6 | 10 | 10 | 4 | 10 |
| Atom | 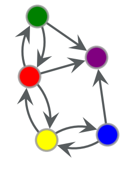 | 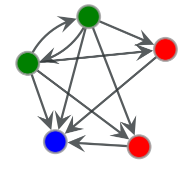 | 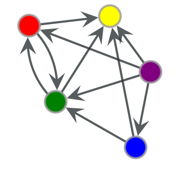 | 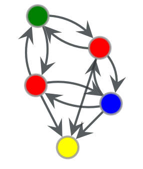 | 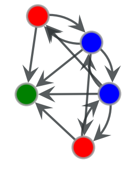 | 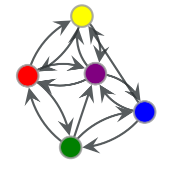 |
| $n_m$ | 5 | 18 | 10 | 5 | 8 | 5 |

Table 6: Atoms in the subgraph MAP-configuration for the C.Elegans neural network and their respective frequencies ($n_m$).

$m$-subgraphs in the inferred configuration $C_\Sigma$ are replaced by single edges i.e.:

$$c_m = \Sigma(C_{\Sigma - m}) - \Sigma(C_\Sigma). \tag{22}$$

The normalized $c$-score $\tilde{c}_m$ is then defined as $\tilde{c}_m = \frac{c_m}{\sqrt{\sum_{m'} c_{m'}^2}}$.

The a plot of the normalized c-scores for the 43 metabolic networks is given in Fig. 2. We find that the significance profiles of the metabolic networks to be in remarkable agreement considering that the size of the set of potential motifs included in the analysis is 9,578 i.e. directed motifs of up to size 5.

## 5.4 Protein-Protein interactions in yeast

For the PPI network of yeast we obtain a MAP configuration with 44 non trivial atoms that cover approximately 90% of the edges. The MAP configuration is dominated by atoms in the form cliques and complete bipartite motifs and, other regular atoms with up to three orbits. We also observe several larger sparse atoms that are less regular but occur with lower frequencies.

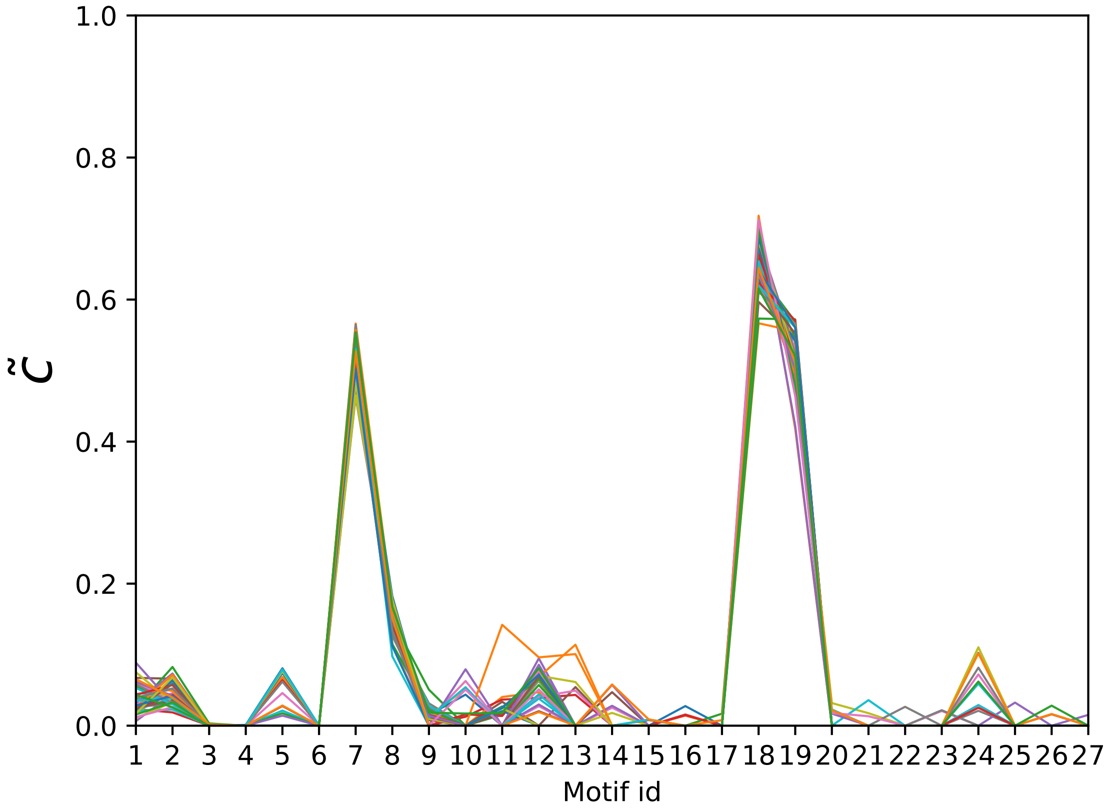


Figure 2: The significance profiles of 43 metabolic networks. The corresponding motifs can be found in Table 7

.

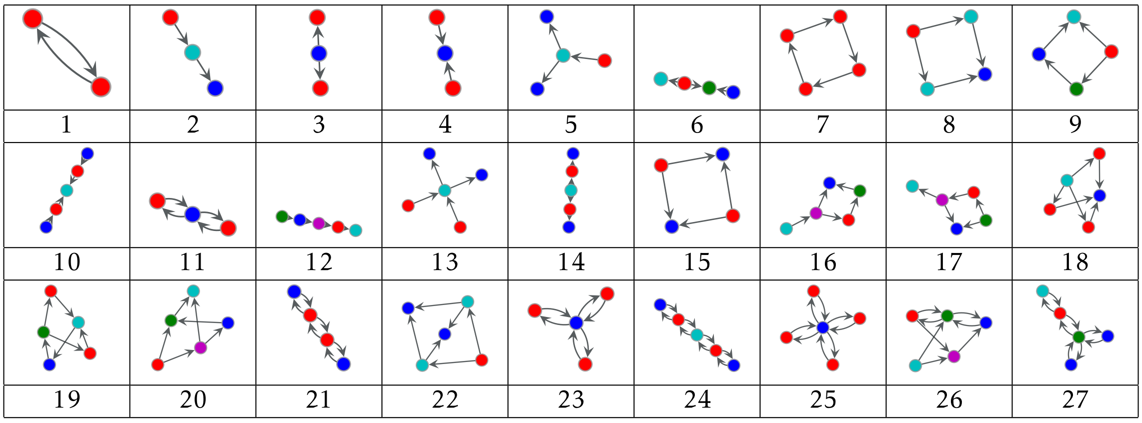

| | | | | | | | | |
|---|---|---|---|---|---|---|---|---|
| 1 | 2 | 3 | 4 | 5 | 6 | 7 | 8 | 9 |
| 10 | 11 | 12 | 13 | 14 | 15 | 16 | 17 | 18 |
| 19 | 20 | 21 | 22 | 23 | 24 | 25 | 26 | 27 |

Table 7: The atoms found in 43 metabolic networks. IDs correspond to the x-axis of the plot in figure 2.

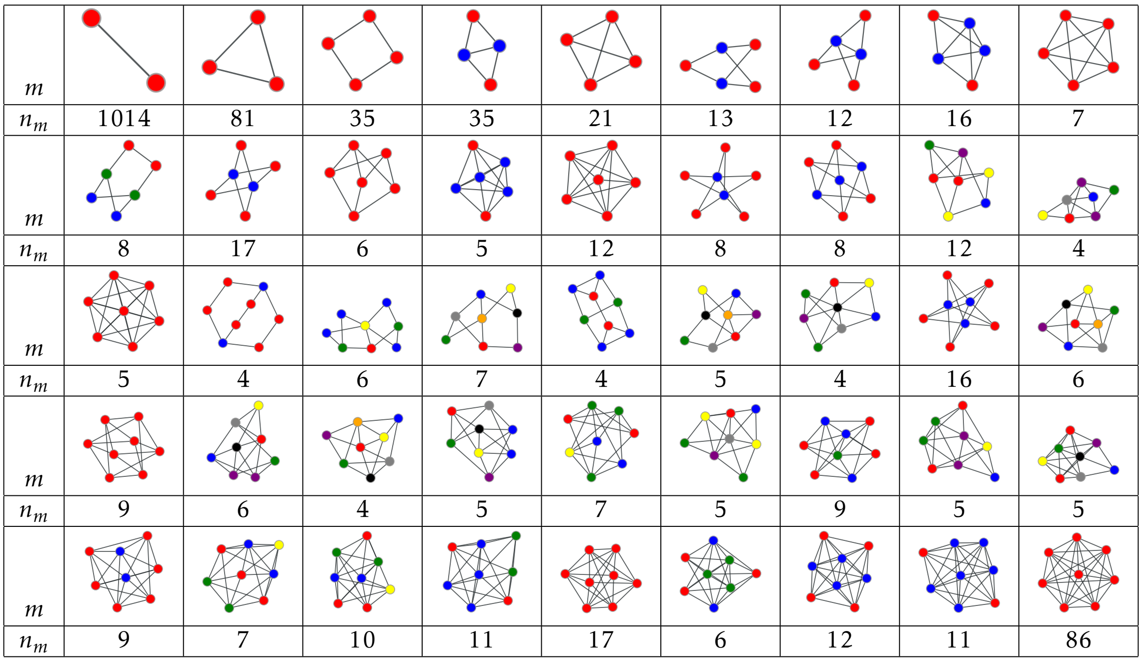

| | | | | | | | | | |
|---|---|---|---|---|---|---|---|---|---|
| $m$ | | | | | | | | | |
| $n_m$ | 1014 | 81 | 35 | 35 | 21 | 13 | 12 | 16 | 7 |
| $m$ | | | | | | | | | |
| $n_m$ | 8 | 17 | 6 | 5 | 12 | 8 | 8 | 12 | 4 |
| $m$ | | | | | | | | | |
| $n_m$ | 5 | 4 | 6 | 7 | 4 | 5 | 4 | 16 | 6 |
| $m$ | | | | | | | | | |
| $n_m$ | 9 | 6 | 4 | 5 | 7 | 5 | 9 | 5 | 5 |
| $m$ | | | | | | | | | |
| $n_m$ | 9 | 7 | 10 | 11 | 17 | 6 | 12 | 11 | 86 |

Table 8: The atoms found in MAP configuration of the PPI network of yeast together with their respective counts.

## 5.5 Gene regulatory network

Next we consider the gene interaction network between recombinant antigen genes from the malaria parasite *P. falciparum* in a highly variable region in the DBLa domain of the var protein (13). Nodes are genes, and edges indicate that two genes share a substring of statistically significant length. The MAP configuration of the malaria network contains 25 nontrivial patterns that cover more than 90% of the edges. Besides a large number of cliques the MAP configuration consists mostly of highly regular subgraphs with up two to four orbits.

## 5.6 Budapest reference connectome

Finally, we consider the undirected reference connectome of the human brain that is the derived from MRI scans of 477 people (14). The MAP configuration of the undirected connectome contains 37 nontrivial atoms that cover approximately 85% of the edges. The MAP configuration contains many large cliques along with densely connected atoms that have up to four orbits. Similar to the gap junction networks we also find 4 cycles and triangles and atoms that consist of

| | | | | | | | | |
|---|---|---|---|---|---|---|---|---|
| 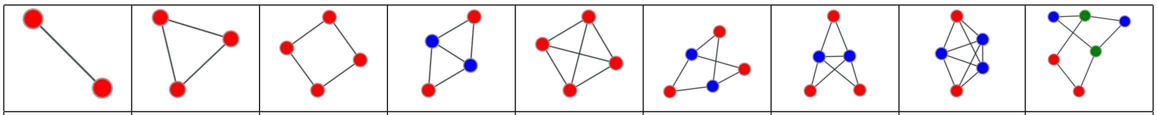 | | | | | | | | |
| 232 | 9 | 9 | 9 | 4 | 11 | 4 | 8 | 8 |
| 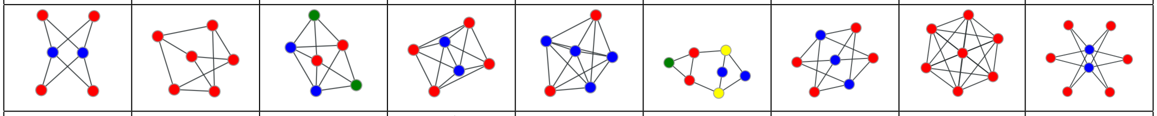 | | | | | | | | |
| 5 | 10 | 8 | 4 | 7 | 5 | 3 | 7 | 3 |
| 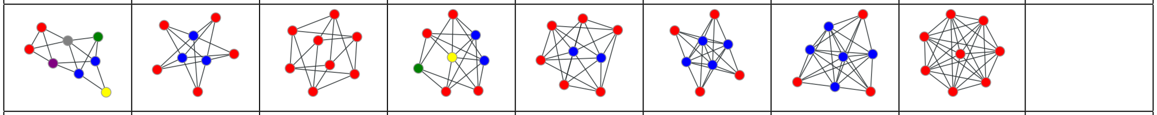 | | | | | | | | |
| 2 | 5 | 6 | 8 | 7 | 9 | 6 | 27 | |

Table 9: The atoms found in a genetic network of the malaria parasite along with their respective counts ($n_m$) in the MAP configuration.

| | | | | | | | | |
|---|---|---|---|---|---|---|---|---|
| $m$ | 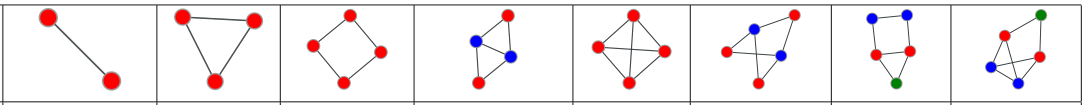 | | | | | | | |
| Id | 0 | 1 | 2 | 3 | 4 | 5 | 6 | 7 |
| $n_m$ | 608 | 11 | 20 | 12 | 2 | 18 | 11 | 8 |
| $m$ | 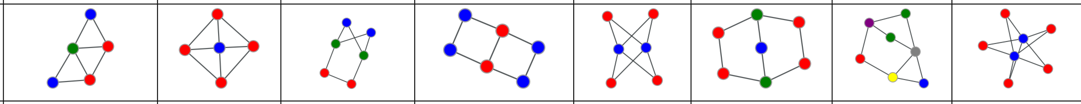 | | | | | | | |
| Id | 8 | 9 | 10 | 11 | 12 | 13 | 14 | 15 |
| $n_m$ | 5 | 23 | 11 | 7 | 18 | 3 | 5 | 7 |
| $m$ | 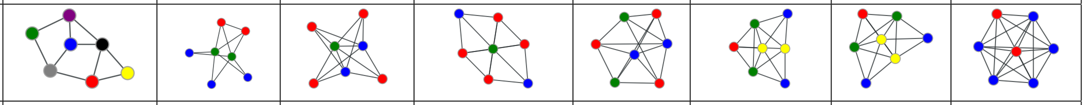 | | | | | | | |
| Id | 16 | 17 | 18 | 19 | 20 | 21 | 22 | 23 |
| $n_m$ | 3 | 8 | 4 | 3 | 7 | 6 | 4 | 9 |
| $m$ | 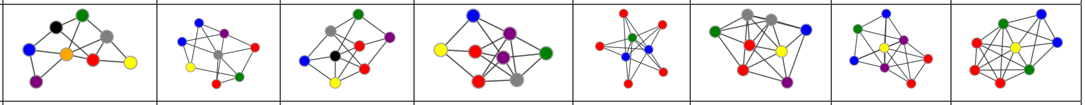 | | | | | | | |
| Id | 24 | 25 | 26 | 27 | 28 | 29 | 30 | 31 |
| $n_m$ | 4 | 4 | 7 | 8 | 6 | 10 | 3 | 5 |
| $m$ | 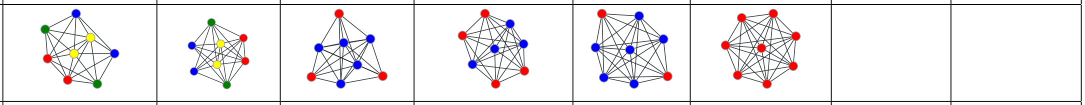 | | | | | | | |
| Id | 32 | 33 | 34 | 35 | 36 | 37 | | |
| $n_m$ | 5 | 4 | 4 | 7 | 4 | 20 | | |

Table 10: Atoms found in the MAP configurations of the Budapest reference connectome of the human brain together with their respective counts in the MAP configuration ($n_m$).

regular combinations of these. The MAP configuration also contains large, sparse and irregular atoms which however occur in smaller numbers.

## 5.7 Directed connectome

A plot MAP configuration of the directed connectome analysed in the main paper is given in Figure 3.

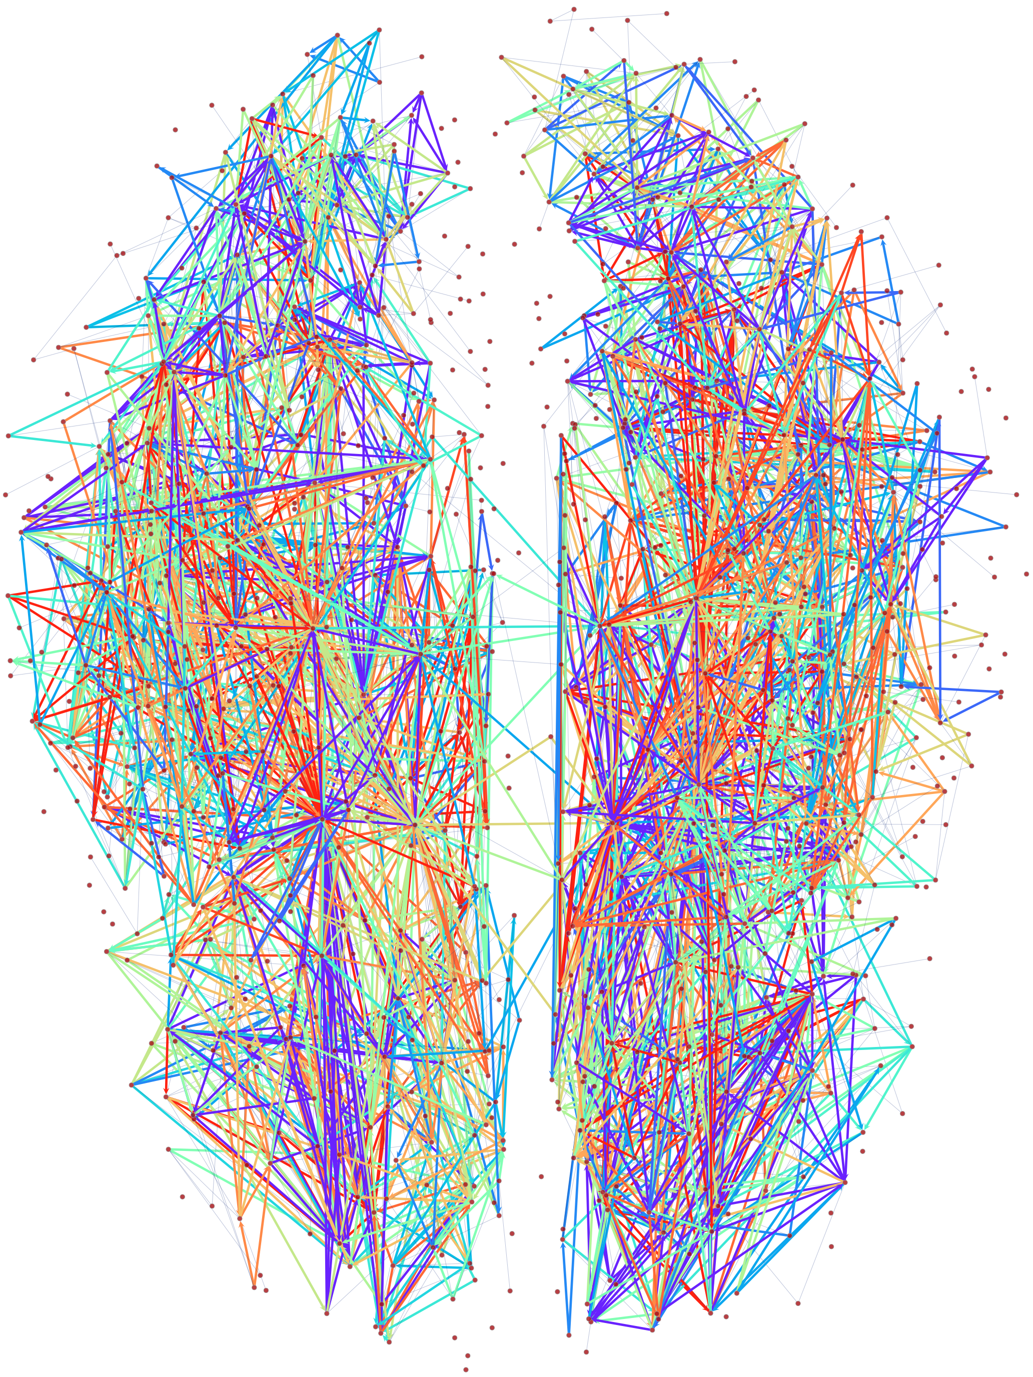

Figure 3: Visualization of the directed brain connectome with edges coloured according the atomic subgraphs they are contained in. Node positions reflect physical locations of brain regions in a 2D projection.

# References


[1] A. E. Wegner and S. Olhede, "Atomic subgraphs and the statistical mechanics of networks," *Physical Review E*, vol. 103, p. 042311, 4 2021.

[2] B. Karrer and M. E. J. Newman, "Random graphs containing arbitrary distributions of sub-

graphs," *Physical Review E*, vol. 82, no. 6, p. 66118, 2010.

[3] G. Bianconi, "Entropy of network ensembles," *Physical Review E*, vol. 79, no. 3, p. 36114, 2009.

[4] E. A. Bender and J. T. Butler, "Asymptotic Aproximations for the Number of Fanout-Free Functions," *IEEE Transactions on Computers*, vol. 27, no. 12, 1978.

[5] J. Rissanen, "Universal coding, information, prediction, and estimation," *IEEE Transactions on Information Theory*, vol. 30, pp. 629–636, 7 1984.

[6] B. D. McKay, "The nauty page," *Computer Science Department, Australian National University, 2004 http://cs. anu. edu. au/bdm/nauty*, 2004.

[7] V. Chvatal, "A greedy heuristic for the set-covering problem," *Mathematics of operations research*, vol. 4, no. 3, pp. 233–235, 1979.

[8] A.-L. Barabási and R. Albert, "Emergence of scaling in random networks," *science*, vol. 286, no. 5439, pp. 509–512, 1999.

[9] P. Erdös and A. Rényi, "On the evolution of random graphs," *Publ. Math. Inst. Hungar. Acad. Sci*, vol. 5, pp. 17–61, 1960.

[10] J. G. White, E. Southgate, J. N. Thomson, S. Brenner, *et al.*, "The structure of the nervous system of the nematode caenorhabditis elegans," *Philos Trans R Soc Lond B Biol Sci*, vol. 314, no. 1165, pp. 1–340, 1986.

[11] H. Jeong, B. Tombor, R. Albert, Z. N. Oltvai, and A.-L. Barabási, "The large-scale organization of metabolic networks," *Nature*, vol. 407, no. 6804, pp. 651–654, 2000.

[12] A. E. Wegner, "Subgraph covers: An information-theoretic approach to motif analysis in networks," *Physical Review X*, vol. 4, no. 4, p. 041026, 2014.

[13] D. B. Larremore, A. Clauset, and C. O. Buckee, "A network approach to analyzing highly recombinant malaria parasite genes," *PLoS computational biology*, vol. 9, no. 10, p. e1003268, 2013.

[14] B. Szalkai, C. Kerepesi, B. Varga, and V. Grolmusz, "The Budapest Reference Connectome Server v2.0," *Neuroscience Letters*, vol. 595, pp. 60–62, 5 2015.
